# Supplementary material for: To Clip or not to Clip: the Dynamics of SGD with Gradient Clipping in High-Dimensions
Source: arXiv:2406.11733 source file (2024-10-06)
Supplement: Supplementary file 1 [file plots_of_thresholds.tex]

\section{Additional plots of \texorpdfstring{\eqref{eq:clip_stability_criterion}}{CSC}}
\label{sec:plots_of_thresholds}

This section is devoted to exploring the two important criterion that we have identified: the \eqref{eq:clip_stability_criterion} and the \eqref{eq:clip_comparison_criterion}. Recall that, \eqref{eq:clip_stability_criterion} describes when clipping results in a algorithm with a higher stability threshold while \eqref{eq:clip_comparison_criterion} describes when clipping can be capable of actually improving the performance of SGD. 

The give some intuition, we provide some plots of these thresholds over various type of noise distributions while the data is assumed to be Gaussian of any covariance.

\begin{figure}[H]
    \centering
    \begin{subfigure}[b]{0.4\textwidth}
        \centering
        \includegraphics[width=\textwidth]{figs/stab_gau_1to6.png}
        \caption
        {Gaussian noise}          
    \end{subfigure}
    \hfill
    \begin{subfigure}[b]{0.4\textwidth}  
        \centering 
        \includegraphics[width=\textwidth]{figs/stab_uni_1to6.png}
        \caption{Uniform noise}  
    \end{subfigure}
    \vskip\baselineskip
    \begin{subfigure}[b]{0.4\textwidth}   
        \centering 
        \includegraphics[width=\textwidth]{figs/stab_rad_1to6.png}
        \caption{Rademacher-type noise}    
    \end{subfigure}
    \hfill
    \begin{subfigure}[b]{0.4\textwidth}   
        \centering 
        \includegraphics[width=\textwidth]{figs/stab_exp_1to6.png}
        \caption{Symmetric exponential noise}      
    \end{subfigure}
    \caption{A comparison of the clipped-stability-criterion \eqref{eq:clip_stability_criterion} for Gaussian data of any covariance and differing noise distributions. The $x$-axis varies across $\noistd$ while the $y$-axis varies over $c$ while the risk is held constant at $1$. The Rademacher-type noise is describe in Theorem \ref{thm:clip_comparison_rademacher}.}    \label{fig:stability_thresholds}
\end{figure}
